# Supplementary material for: Quantum-enhanced magnetometry by phase estimation algorithms with a single artificial atom
Source: arXiv:1801.02230 source file (2018-05-07)
Supplement: Supplementary file 1 [file Supplementary_Information.pdf]

# Supplementary Information for "Quantum-enhanced magnetometry by phase estimation algorithms with a single artificial atom"

S. Danilin, A. V. Lebedev, A. Vepsäläinen, G. B. Lesovik, G. Blatter, G. S. Paraoanu

## S1. The sample and the qubit detection scheme

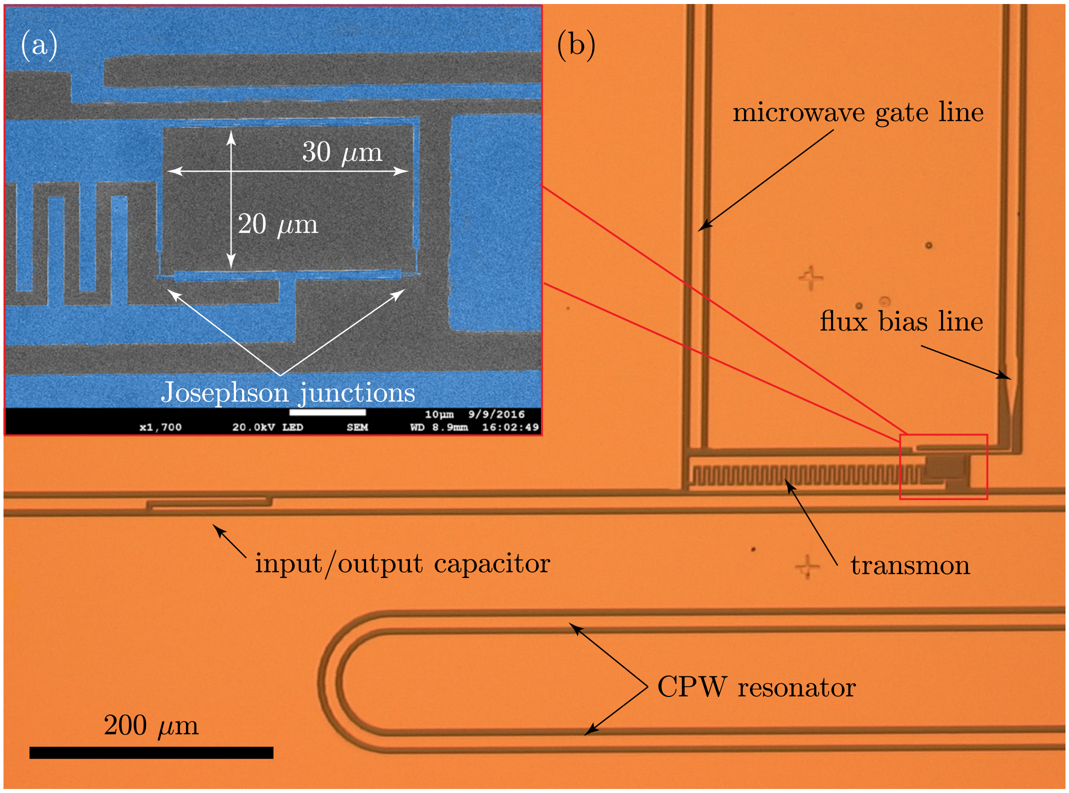


**Figure 1. (a)** SEM image of the transmon SQUID loop (false colors). **(b)** Optical microphotograph of the sample.

The sample (see Fig. (1)) is fabricated using the standard double-angle shadow deposition technique where first 30 nm and then 60 nm of aluminum was evaporated on the pure high resistive silicon substrate at angles of $\pm 30^\circ$ correspondingly. This is followed by the lift-off process.

The measurement of the qubit state is realized with homodyne detection by sending a 2 $\mu$s probe pulse of a rectangular shape with a $\nu_{\rm pr}$ carrier frequency into the resonator immediately after the second $\pi/2$ pulse of the Ramsey sequence. The reflected back from the resonator signal is down-converted to a slowly varying responce $r(t)$, which is recorded by a data acquisition card with 1 ns resolution. The calibration of the readout scheme is done at a fixed flux value $\Phi_{\rm cal}$, corresponding to a dc-voltage bias $V_{\rm cal} = 0.98$ V at the qubit flux bias line where the frequency mismatch $\Delta\omega(\Phi_{\rm cal})$ approximately vanishes. At this specific flux point we prepare the qubit in the ground $|0\rangle$ and in the excited state $|1\rangle$ and record the corresponding response signals $r_{0,1}(t)$. For each of these basis states we average over $N_{\rm cal} = 30 \times 65000$ separate response curves and find the averaged time traces $\bar{r}_{0,1}(t)$. This averaging is done in order to increase the signal-to-noise ratio. In order to optimize the readout scheme we sweep the probe pulse frequency $\nu_{\rm pr}$ and find the point where the area between ground and excited state response curves

$$A_{01} = \int_{t_0}^{t_1} dt\, |\bar{r}_0(t) - \bar{r}_1(t)| \qquad (1)$$

is maximal. In our setup the optimal probe pulse frequency was $\nu_{\rm pr} = 5.1254$ GHz, and we take $t_0 = 80$ ns and $t_1 = 1800$ ns counted from the beginning of the probe pulse.

For a qubit prepared in an arbitrary superposition $|\psi\rangle = \alpha|0\rangle + \beta|1\rangle$ the probe pulse projects the qubit either into the ground or excited state. The corresponding response curve $r(t)$ is either $\bar{r}_0(t) + \nu(t)$ or $\bar{r}_1(t) + \nu(t)$ if the qubit was projected into the

ground or excited state. Here $\nu(t)$ is the noise in the measurement setup, which includes the added noise of the amplifiers chain (a low-noise cryogenic amplifier placed at the 4K plate of the dilution refrigerator and two microwave room temperature amplifiers). Our readout scheme returns a variable

$$h = \frac{1}{A_{01}} \int_{t_0}^{t_1} dt \left(r(t) - \bar{r}_0(t)\right) \text{sgn}\left(\bar{r}_1(t) - \bar{r}_0(t)\right) \equiv s + \xi, \tag{2}$$

where $s$ is a discrete random variable which gets values 0 or 1 with probabilities $|\alpha|^2$ and $|\beta|^2$ correspondingly; $\xi$ is a random Gaussian variable

$$\xi = \frac{1}{A_{01}} \int_{t_0}^{t_1} dt\, \nu(t) \text{sgn}\left(\bar{r}_1(t) - \bar{r}_0(t)\right). \tag{3}$$

We prepare and measure the qubit $N$ times and collect $N$ readouts $h_i$, $i = 1, \ldots N$. Then, according to a central limit theorem at large $N$ the averaged readout $h_N = \frac{1}{N} \sum_{i=1}^{N} h_i$ is a normally distributed random variable,

$$p(h_N) = \frac{1}{\sqrt{2\pi}\sigma_N} \exp\left(-\frac{(h_N - |\beta|^2)^2}{2\sigma_N^2}\right), \qquad \sigma_N^2 = \frac{\sigma_1^2 + |\alpha|^2|\beta|^2}{N}, \qquad \sigma_1^2 = \langle \xi^2 \rangle. \tag{4}$$

For a large $N \gg 1$, the distribution function $p(h_N)$ is peaked near the probability of the excited state $|\beta|^2$. The noise variance $\sigma_1^2$ can be measured directly by reading out $h$ for the qubit prepared either in the ground $|\alpha|^2 = 1$ or excited $|\beta|^2 = 1$ states. It turns out that in our setup we have $\sigma_1^2 \approx 1.5$.

## S2. Qubit passport measurement

We refer to the measured value of the readout variable $h_N$ after N Ramsey sequences with a delay $\tau$ for a given flux $\Phi$ as a qubit's 'passport' function $P_p(\tau, \Phi) = h_N(\tau, \Phi)$. We use for the passport measurement $N = 65000$ and digitise the parameter space $(\tau, \Phi)$ into 241 time delay points $\tau_n$, $n = 0, \ldots 240$, and 161 magnetic flux points $\Phi_m$, $m = 1, \ldots 161$. The time delay poins are separated by 2 ns time step with $\tau_0 = 0$ ns and $\tau_{240} = 480$ ns. The magnetic flux $\Phi$ is controlled by a dc-voltage bias applied to the flux bias line. This voltage bias is produced by an Agilent 33500B waveform generator with high stability OCXO timebase, which has 12 mV absolute-voltage accuracy at the 1 V output level. The precision of this device is well below 0.2 mV, which is the step between the chosen 161 equidistant voltage values $V_m$, $m = 1, \ldots, 161$ with $V_1 = 0.977$ V and $V_{161} = 1.009$ V. In our experiment we keep the drive frequency of Ramsey sequence microwave pulses constant at $\omega_{\text{dr}} = 2\pi \times 7.246$ GHz. At every flux value $\Phi(V_m)$ we measure a passport curve $P_p(\tau_n, \Phi(V_m))$.

We fit the measured passport curves $P_p(\tau_n, \Phi(V_m))$ by two types of fit functions: one with an exponential decay,

$$P_m^{(exp)}(\tau) = \alpha_m + \beta_m \exp(-\gamma_m \tau) \cos\left(\omega_m \tau + \varphi_m\right), \tag{5}$$

and another with a Gaussian decay function combined with an exponential relaxation factor,

$$P_m^{(gauss)}(\tau) = \alpha_m + \beta_m \exp(-\tau/(2T_1) - (\tau/T_\phi)^2) \cos\left(\omega_m \tau + \varphi_m\right). \tag{6}$$

The fit results at different bias voltage points are shown in Figs.2a and 2b at the sweet spot of the qubit spectrum and at the bias point, where our metrological experiment was done. For our sample we can not distinguish between two fit functions Eq. (5) and (6) and in the following we use an exponential decay fit function given by Eq. (5).

It turns out that among five fitting parameters $\alpha_m$, $\beta_m$, $\gamma_m$, $\omega_m$ and $\varphi_m$, $m = 1, \ldots, 161$ the decay rate $\gamma_m$ is almost insensitive to the flux $\Phi(V_m)$ and we keep it constant at $\gamma_m^{-1} = 260 \pm 30$ ns. We observe a clear linear dependence of the frequency $\omega_m$ and phase $\varphi_m$ on the voltage bias, see Fig. 3a and 3b. The corresponding linear fits are,

$$\omega_m = 2\pi \times \left(423 V_m - 411\right) \text{MHz}, \qquad \varphi_m = 78.6 V_m - 76.5. \tag{7}$$

The observed linear dependence of $\omega_m$ is natural: we operate the qubit in a linear regime where its transition frequency $\omega_{01}(\Phi)$ depends linearly on the magnetic flux and hence on the applied voltage $V$. From the spectroscopy measurements of the transition frequency $\omega_{01}$ one can estimate the sensitivity $\frac{d\omega_{01}}{dV} \approx -2\pi \times 422$ MHzV$^{-1}$ at $V = 0.98$ V, which is in a good agreement with a linear fit (7). The phase $\varphi_m$ is mostly accumulated during the application of two $\pi/2$ microwave pulses of the Ramsey sequence,

$$\varphi_m = \omega_m \tau_0 + \delta\varphi, \tag{8}$$

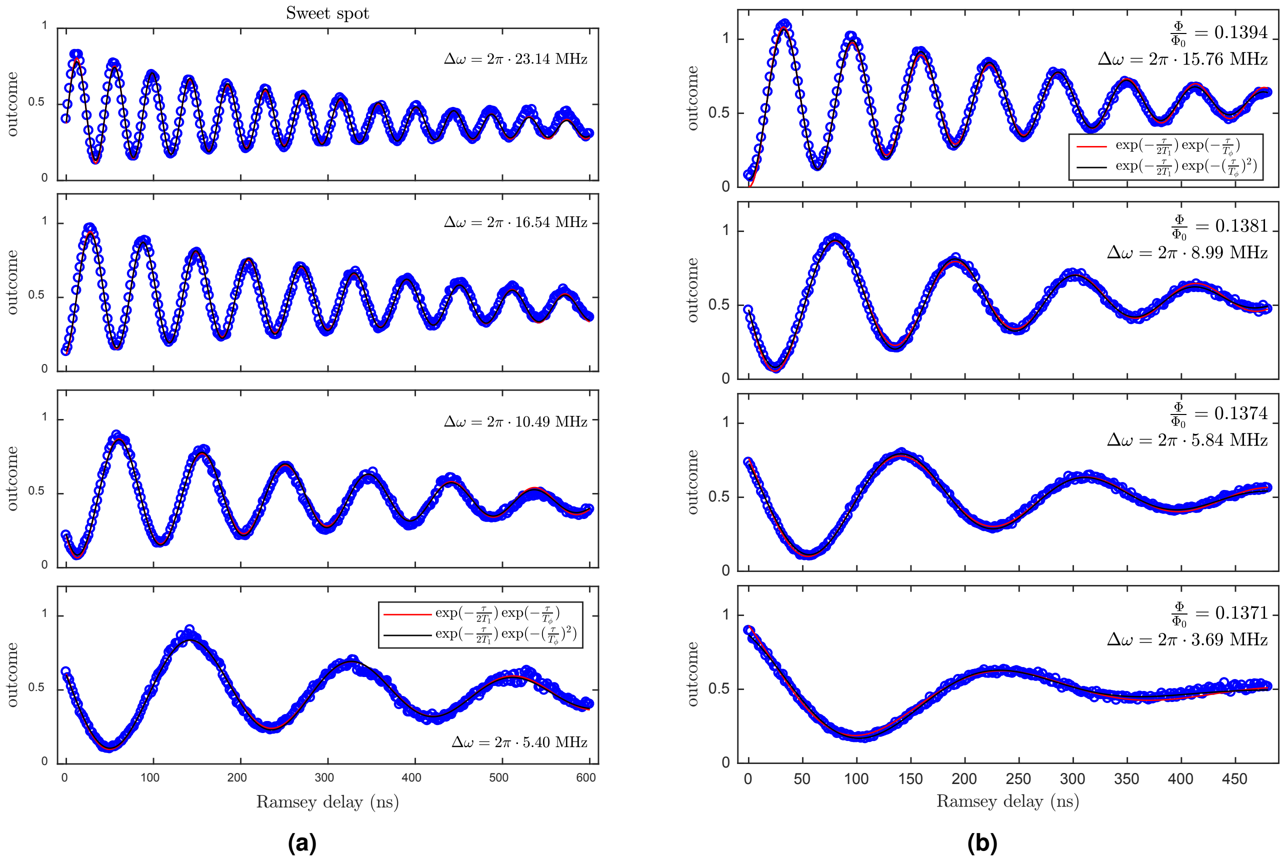


**Figure 2.** **a)** Measurement of a free-induction decay near the sweet spot of the qubit spectrum at four different flux values corresponding to the frequency detunings: $\Delta\omega = \omega_{\mathrm{dr}} - \omega_{01}(\Phi)$. The observed experimental curves are fitted by the exponential decay function with (red) and the Gaussian decay function (black). The pure dephasing times for an exponential decay model are $T_\phi = 1431, 1042, 1374$ and 887ns (from top to bottom) while for the Gaussian decay model we have $T_\phi = 853, 696, 850$ and 678ns. **b)** Measurement of a free-induction decay near the bias point at four different magnetic flux values from the range used for the "passport" measurement shown in the Fig. (1b) of the article main text. The red lines are the fits with the exponential decay $T_\phi = 567, 491, 450$ and 259ns (from top to bottom), the black lines are the Gaussian fits $T_\phi = 453, 424, 417$ and 282ns.

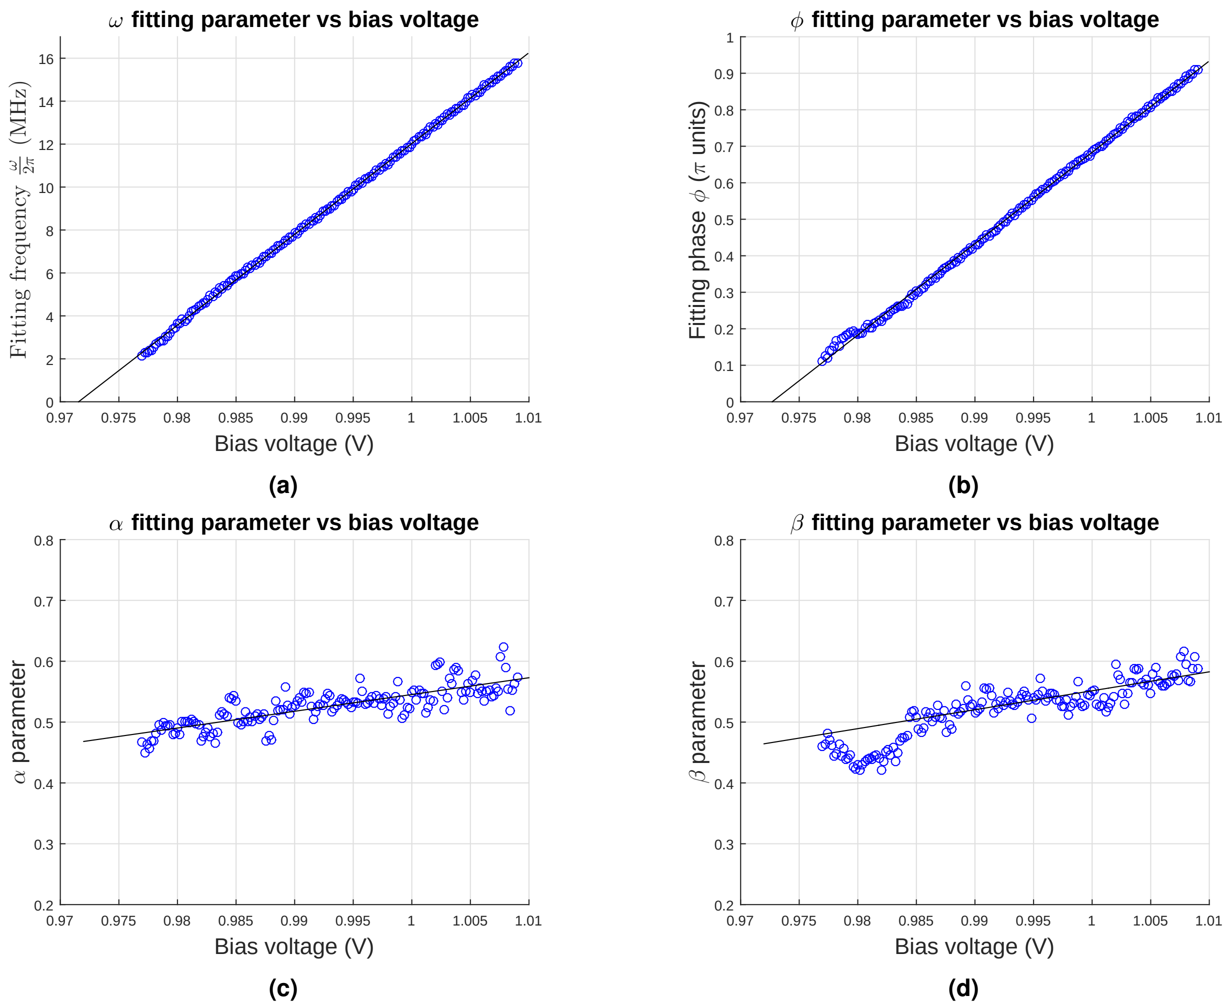


**Figure 3.** The dependencies of the Eq. (5) fitting parameters (blue curves) on the flux bias voltage and their linear fits (solid lines).

where $\tau_0$ is a time parameter which defines an effective duration of two $\pi/2$ microwave pulses, $\delta\varphi$ is a residual flux independent phase. Then $\tau_0 = \frac{d\varphi_m}{d\omega_m} \approx 31.6$ ns. The residual phase $\delta\phi$ is normally distributed with a mean value $-0.095$ and a standard deviation 0.055.

The fitting parameters $\alpha(V_m)$ and $\beta(V_m)$ have a weak linear dependence, see Fig. 3c and 3d, $\alpha_m = 2.75V_m - 2.21$ and $\beta_m = 3.11V_m - 2.56$. Both $\alpha$ and $\beta$ have the same tendency: these parameters increase as the voltage growths. We argue that the origin of this dependence is the CPW resonator-qubit coupling. Indeed, the bare eigenfrequency of the resonator $\omega_{\rm res}$ is renormalized by the qubit coupling: $\omega_{\rm res} \to \omega_{\rm res} - \chi_{12}/2$, where $\chi_{12}$ is a resonator's partial dispersive shift,

$$\chi_{12} = \frac{2g_{01}^2}{\omega_{01}(\Phi) - \omega_C - \omega_{\rm res}}, \tag{9}$$

where $g_{01} \sim 2\pi \times 100$ MHz is the resonator-qubit coupling constant found form the spectroscopy measurement, $\omega_C = 2\pi \times 299$ MHz is a frequency associated with the charging energy of the transmon: $\omega_C = E_C/\hbar$. In the measured flux interval $[\Phi(V_1), \Phi(V_{161})]$ the qubit transition frequency $\omega_{01}(\Phi)$ varies within a $\Delta\omega_{01} \approx -2\pi \times 13.5$MHz interval. Then according to Eq. (9) the resonator's frequency changes within

$$\Delta\omega_{\rm res}(\Phi) = \frac{1}{2}\frac{\partial\chi_{12}}{\partial\omega_{01}}\Delta\omega_{01} = -\frac{g_{01}^2}{(\omega_{01}(\Phi) - \omega_C - \omega_{res})^2}\Delta\omega_{01} \approx 2\pi \times 41\,\text{kHz} \tag{10}$$

that is compatible with the resonance width $\sim 550$ kHz. In the passport measurement the calibration of the readout scheme is done at a fixed flux value corresponding to $V_{\rm cal} = 0.98$ V. During the passport measurement the flux changes from the calibration point and hence changes the resonator's frequency as well. As a result, at a given flux value $\Phi(V)$ the true calibration response traces $\bar{r}_0(t|V)$ and $\bar{r}_1(t|V)$ are different from the response traces $\bar{r}_0(t|V_{\rm cal})$ and $\bar{r}_1(t|V_{\rm cal})$ used in the readout scheme, see Supplementary Information 1. Therefore, the readout variable, see Eq. (2), might systematically deviate from the true probability of the excited state for the fluxes far away from the calibration point.

These arguments are confirmed by a direct measurement of the resonator's responses at the probe frequency $\nu_{\rm pr} =$ 5.12540 GHz used in the experiment and at a frequency shifted by 50 kHz, namely at 5.12545 GHz. The response traces are indeed different, see Fig. 4, and therefore the readout variable $h_N$ for the qubit prepared in the excited state gets a value higher than 1,

$$h_N = \frac{\int_{t_0}^{t_1} dt(\bar{r}_1(t|V) - \bar{r}_0(t|V_{\rm cal}))\text{sgn}(\bar{r}_1(t|V_{\rm cal}) - \bar{r}_0(t|V_{\rm cal}))}{\int_{t_0}^{t_1} dt|\bar{r}_1(t|V_{\rm cal}) - \bar{r}_0(t|V_{\rm cal})|} \approx 1.15 > 1. \tag{11}$$

Hence, at a given flux the readout variable $h_N$ is not a true probability of the excited state, but rather a quantity which is proportional to it.

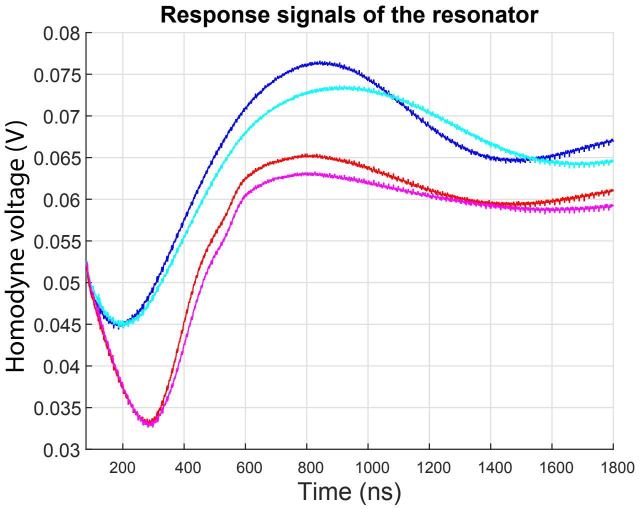


**Figure 4.** Homodyne response traces measured at a probe frequency 5.12540 GHz (for the ground state (blue curve) and the excited state (red curve)), and their counterparts measured at the shifted probe frequency of 5.12545 GHz (for the ground state (cyan curve) and the excited state (magenta curve)).

## S3. Modified Kitaev phase estimation algorithm

Here we describe in detail our modified versions of the Kitaev and the Fourier phase estimation algorithms. Both algorithms exploit the pre-measured qubit's discrete passport function $P_p(\tau_n, \Phi_m)$. The elementary subroutine used in both algorithms is the Bayesian update procedure,

**function** $BayesianUpdate(\mathscr{P}, \tau)$
  $h_N \leftarrow GetOutcome(\tau, N)$;
  $\forall m:\ \ \mathscr{P}(\Phi_m) \leftarrow \mathscr{P}(\Phi_m) \exp\Big(-\big(h_N - P_p(\tau, \Phi_m)\big)^2/2\sigma_N^2\Big)$;
  $\forall m:\ \ \mathscr{P}(\Phi_m) \leftarrow \mathscr{P}(\Phi_m)/\sum_n \mathscr{P}(\Phi_n)$;
  **return** $\mathscr{P}(\Phi_m)$;
**end function**

It takes as an input two parameters: i) the current flux probability distribution $\mathscr{P}(\Phi_m)$ and ii) Ramsey delay time parameter $\tau$. N sequences of Ramsey pulses with the delay $\tau$ is generated and the value of the readout variable $h_N$ is measured. Then the Bayesian procedure uses the obtained measurement outcome together with the passport function and updates the flux probability distribution according to the Bayes rule. Finally, the updated distribution is normalized.

Our Kitaev phase estimation algorithm has two input parameters: number of successive steps $K$ and a tolerance $\varepsilon > 0$, which defines the accuracy of the procedure at each its step. The algorithm has the form

**function** $KitaevProcedure(K, \varepsilon)$
  $S = [1, \ldots, 161]$;
  $\tau = 0$;
  **for** $k = 1, \ldots, K$ **do**
    $\forall m \in S:\ \ \mathscr{P}(\Phi_m) = 1/\mathscr{N}(S)$;
    $\forall m \notin S:\ \ \mathscr{P}(\Phi_m) = 0$;
    **repeat**
      $\mathscr{P} \leftarrow BayesianUpdate(\tau, N)$;
      $S = S_{0.5}^{>} \cup S_{0.5}^{<}$;
    **until** $\sum_{m \in S_{0.5}^{<}} \mathscr{P}(\Phi_m) > \varepsilon$
    $S \leftarrow S_{0.5}^{>}$;
    $\tau \leftarrow NextOptimalDelayKitaev(S)$;
  **end for**
  **return** $\text{argmax}\mathscr{P}(\Phi_m)$;
**end function**

In the beginning, the algorithm initializes a uniform discrete flux probability distribution $\mathscr{P}(\Phi_m)$ for a given initial set of indexes $m \in S = [1, \ldots, 161]$ which enumerate flux values $\Phi_m$ used for the passport measurement. At the first step ($k = 1$) the algorithm repeats the Bayesian update procedure with a minimal delay $\tau = 0$ until the probability distribution $\mathscr{P}(\Phi_m)$ squeezes into an index subset $m \in S_{0.5}^{>} \subset S$ which is twice smaller than the original set $S$: $\mathscr{N}(S_{0.5}^{>}) = \lceil \mathscr{N}(S)/2 \rceil$ ($\lceil x \rceil \geq x$ denotes the nearest integer bigger than the number $x$)

$$S = S_{0.5}^{>} \cup S_{0.5}^{<}, \qquad \mathscr{P}(\Phi_m) > \mathscr{P}(\Phi_n) \quad \forall m \in S_{0.5}^{>}, \quad \forall n \in S_{0.5}^{<}, \tag{12}$$

where $\mathscr{N}(S)$ denotes the number of elements in the set $S$. The update procedure repeats until the sum of the probabilities $\sum_{m \in S_{0.5}^{<}} \mathscr{P}(\Phi_m)$ gets smaller than $\varepsilon$. Then the algorithm assumes that the measured flux is located within a set $\Phi_m$, $m \in S_{0.5}^{>}$ with probability $1 - \varepsilon$ and resets the flux probability distribution to be uniform on the remaining set of indexes. In our version of the Kitaev algorithm, the time delay $\tau$ of the Ramsey sequence serves as an adaptive parameter. Its value is dynamically adjusted for the next steps $k > 1$ of the procedure by a function

**function** $NextOptimalDelayKitaev(S)$
  **for** $\tau = 0, \ldots, T_2$ **do**
    $\Delta P(\tau) = \max_{m \in S} P_p(\tau, \Phi_m) - \min_{m \in S} P_p(\tau, \Phi_m)$;
  **end for**

**return** argmax$\Delta P(\tau)$;
**end function**

which sweeps the passport function $P_p(\tau, \Phi_m)$ and for every delay $\tau$ finds a probability range $\Delta P(\tau)$ on the set of indexes $m \in S$. The next optimal Ramsey delay corresponds to the delay $\tau$ where the probability range is maximal. After $K$ steps the measured flux value is localized with a probability $(1-\varepsilon)^K$ within a flux interval which is $2^K$ times shorter than the initial flux interval.

## S4. Modified Fourier phase estimation algorithm

Our version of the Fourier phase estimation algorithm has the form

```
function FourierProcedure(K,{ε_1,...,ε_K},τ_s)
    S = [1,...,161];
    ∀m ∈ S :  𝒫(Φ_m) = 1/𝒩(S);
    repeat
        𝒫 ← BayesianUpdate(τ_s,N);
        S = S^>_{0.5} ∪ S^<_{0.5};
    until ∑_{m∈S^<_{0.5}} 𝒫(Φ_m) > ε_1

    S ← S^>_{0.5};

    for k = 2,...,K do
        ∀m ∈ S :  𝒫(Φ_m) = 1/𝒩(S);
        ∀m ∉ S :  𝒫(Φ_m) = 0;
        (τ,A,B) ← NextOptimalDelayFourier(S);

        repeat
            𝒫 ← BayesianUpdate(τ,N);
            p_a = ∑_{m∈A} 𝒫(Φ_m);
            p_b = ∑_{m∈B} 𝒫(Φ_m);
        until min{p_a, p_b} > ε_k

        if p_a > p_b then
            S ← A;
        else
            S ← B;
        end if

    end for
    return argmax𝒫(Φ_m);
end function
```

Differently from the Kitaev algorithm, the Fourier algorithm starts the Bayesian update procedure at some large time delay $\tau_s \sim T_2$. At large time delays the passport function $P_p(\tau, \Phi)$ is not a monotonic function of $\Phi$. As a result, after the first step the flux probability distribution $\mathscr{P}(\Phi_m)$ has several narrow peaks (see the main text). Each peak corresponds to a different alternative in a measured flux value and widths of the peaks define the final measurement accuracy. At the next steps, $k = 2, \ldots, K$ the Fourier procedure discriminates between these alternatives and reveals at the end of the measurement only a single peaked flux distribution. This logic changes the way in which the Fourier algorithm searches for the next optimal delay:

```
function NextOptimalDelayFourier(S)
    N ← 𝒩(S);
    for τ = 0,...,τ_s do
        p = {P_p(τ,Φ_{m_1}) ≥ P_p(τ,Φ_{m_2}) ≥ ··· ≥ P_p(τ,Φ_{m_N})};
        A(τ) ← {m_i,   i = 1,...,[N/2]};
        B(τ) ← {m_i,   i = [N/2]+1,...,N};
```

$\Delta p_{A,B}(\tau) \leftarrow P_p(\tau, \Phi_{[\frac{N}{2}]}) - P_p(\tau, \Phi_{[\frac{N}{2}]+1});$

**end for**

$\tau = \text{argmax}_\tau \Delta p(\tau);$

**return** $(\tau, A(\tau), B(\tau));$

**end function**

The $NextOptimalDelayFourier(S)$ function takes the set of remaining indexes $S$ and sweeps over the passport function. At every time delay $\tau$ it orders the probability values $P(\tau, \Phi_m)$, $m \in S$ and splits $S$ into two approximately equal in size subsets: $S = A \cup B$, where $P_p(\tau, \Phi_{m \in A}) > P_p(\tau, \Phi_{m \in B})$. The optimal time delay $\tau$ corresponds to a delay where the probability distance $\Delta p_{A,B}(\tau) = \min_{m,n} \left[ P_p(\tau, \Phi_{m \in A}) - P_p(\tau, \Phi_{n \in B}) \right]$ between two subsets is maximal. Then the function $NextOptimalDelayFourier(S)$ returns three values: the optimal time delay $\tau$, and two corresponding subsets of indexes $A(\tau)$ and $B(\tau)$. Then the Fourier algorithm runs the Bayesian update procedure at the optimal delay $\tau$ and discriminates between two alternatives for the flux to be localized either in $A$ or in $B$ with an error probability given by the input parameter $\varepsilon_k$. Proceeding in this manner the Fourier algorithm in $K-2$ steps discriminates between the remaining alternatives and finally returns the most probable value of the flux.
